# Supplementary material for: Local Correlation Clustering with Asymmetric Classification Errors
Source: arXiv:2108.05697 source file (2021-08-11)
Supplement: Supplementary file 1 [file ineq-on-F.tex]

%\section{Proof of Claim~\ref{cl:ineq-on-F}}\label{sec:cl:ineq-on-F}
\begin{proof}[Proof of Claim~\ref{cl:ineq-on-F}]
We have
\begin{align*}
F(x_2)-F(x_1) &= \int_{x_1}^{x_2} F'(x) dx\\
&\leq (x_2 - x_1) \max_{x\in [x_1,x_2]}F'(x)\\
&= (x_2 - x_1) \cdot \frac{e^{-\nicefrac{x_1}{R_0}}/R_0}{1-e^{-\nicefrac{R}{2R_0}}}\\
&= (x_2 - x_1) \cdot \frac{
   e^{-\nicefrac{x_1}{R_0}}/R_0
}{
1-\beta^{q+1}
}.
\end{align*}
Since $\beta^{q+1} \leq 1/2$, we have $1/(1-\beta^{q+1})\leq 1+2\beta^{q+1}$. Thus,
\begin{align*}
F(x_2)-F(x_1)&\leq
(x_2 - x_1) \cdot    \frac{e^{-\nicefrac{x_1}{R_0}}}{R_0}\cdot (1+2\beta^{q+1})\\
&< (x_2 - x_1) \cdot    \frac{e^{-\nicefrac{x_1}{R_0}}+2\beta^{q+1}}{R_0}.
\end{align*}
\end{proof}
