# Supplementary material for: Local Correlation Clustering with Asymmetric Classification Errors
Source: arXiv:2108.05697 source file (2021-08-11)
Supplement: Supplementary file 2 [file proof-map-pi.tex]

\section{Proof of Lemma~\ref{lem:function-pi}}\label{sec:proof-map-pi}
\begin{proof}
Note that $\pi_S^{inv}(y)$ is a right inverse for $\pi_S(x)$: $\pi_S(\pi_S^{inv}(y)) = y$ (but not necessarily a left inverse).
Let 
$$I_S(x) = 
\begin{cases}
    1,&\text{if } x\in S\\
    0,&\text{otherwise}
\end{cases}
$$
be the indicator function of set $S$.
Then $\pi_S(x) = \int_0^x I_S(t) dt$ (we use Lebesgue integration here). Since $0\leq I_S(t) \leq 1$, function $\pi_S$ is non-decreasing, $1$-Lipschitz, and absolutely continuous. By the Lebesgue differentiation theorem, $\pi_S(x)$ is almost everywhere differentiable and $\frac{d\pi_S(x)}{dx} = I_S(x)$. Let $X_0 = [0,R]\setminus S$ and $Y_0 = \pi_S(X_0)$. Since $\pi_S$ is absolutely continuous and $I_S(x) = 0$ for $x\in X_0$, we have
$$\mu(Y_0)\leq\int_{X_0}\frac{d\pi_S(x)}{dx}dx = \int_{X_0}I_S(x) dx = 0.$$
Now if $y\notin Y_0$, then $\pi_S(\pi_S^{inv}(y)) = y\notin Y_0$, thus $\pi_S^{inv}(y)\notin X_0$ or, equivalently,
$\pi_S^{inv}(y)\in S$, as required.

Finally, we verify that $\pi_S^{inv}$ is strictly increasing. Consider $a,b \in [0,\mu(S)]$ with $a < b$. Note that $a = \pi_S(\pi_S^{inv}(a))$ and $b = \pi_S(\pi_S^{inv}(b))$. Thus, $\pi_S(\pi_S^{inv}(a))< \pi_S(\pi_S^{inv}(b))$. Since $\pi_S$ is non-decreasing, 
$\pi_S^{inv}(a) < \pi_S^{inv}(b)$.
\end{proof}
